# Supplementary material for: Fractional viscoelastic models for power-law materials
Source: arXiv:2003.07834 ancillary file (2020-07-15)
Supplement: Supplementary file 1 [file Annex_Summary_fractional_models.pdf]

# Fractional viscoelastic models for power-law materials

## Annex: Summary of their constitutive equations, moduli & qualitative behaviours

Bonfanti A, Kaplan JL, Charras G, Kabla A

March 20, 2020

### Content

This document is an annex to “Fractional viscoelastic models for power-law materials” [1]. It presents a classification of the main linear viscoelastic models and provides, for each of them, a constitutive equation and analytical forms of the relaxation, creep and complex moduli in the time domain wherever possible, or in the Laplace domain otherwise. Graphs of these functions are included for provide a qualitative picture of how key rheological parameters influence the response.

These models are integrated in the software package RHEOS [2], and the code used to generate the figures in the document is available in the software repository [3].

### References

1. Bonfanti, A., Kaplan, J. L., Charras, G. & Kabla, A. J. Fractional viscoelastic models for power-law materials. *arXiv*. doi:2003.07834 (2020).
2. Kaplan, J. L., Bonfanti, A. & Kabla, A. RHEOS.jl – A Julia Package for Rheology Data Analysis. *Journal of Open Source Software* (2019).
3. Kaplan, J. L., Bonfanti, A. & Kabla, A. RHEOS.jl. *GitHub repository* <https://github.com/JuliaRheology/RHEOS.jl> (2020).

## 1 Spring-pot

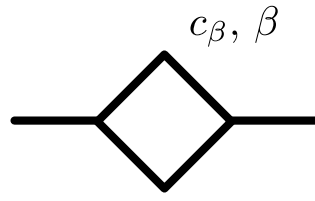

### Constitutive equation

$$\sigma(t) = c_\beta \frac{d^\beta \epsilon(t)}{dt^\beta} \text{ for } 0 \leq \beta \leq 1$$

### Relaxation modulus

$$G(t) = \frac{c_\beta}{\Gamma(1-\beta)} t^{-\beta}$$

### Creep modulus

$$J(t) = \frac{1}{c_\beta \Gamma(1+\beta)} t^\beta$$

### Complex modulus

$$G^*(\omega) = c_\beta (i\omega)^\beta$$

### Storage modulus

$$G'(\omega) = c_\beta \omega^\beta \cos\left(\frac{\pi}{2}\beta\right)$$

### Loss modulus

$$G''(\omega) = c_\beta \omega^\beta \sin\left(\frac{\pi}{2}\beta\right)$$

---

### Special cases

- Spring:  $\beta = 0$

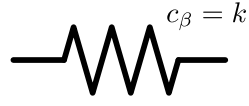

- Dashpot:  $\beta = 1$

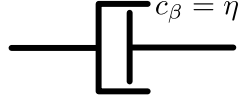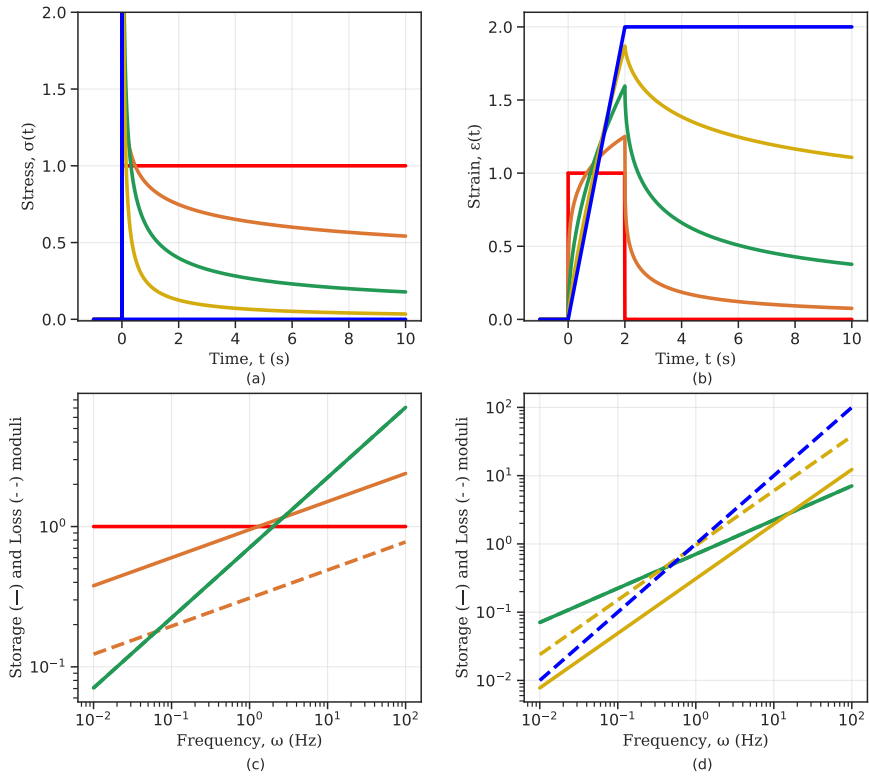

Figure 1: Springpot behaviour for varying  $\beta$ . Color reference  $\beta$  values are red (0.0), orange (0.3), yellow (0.5), green (0.7) and blue (1.0). (a) Relaxation response to step loading. (b) Creep response to step loading and unloading. (c) and (d) Storage (solid line) and loss (dashed line) moduli for the main values of  $\beta$  with colors ascribed above.

## 2 Fractional Maxwell model

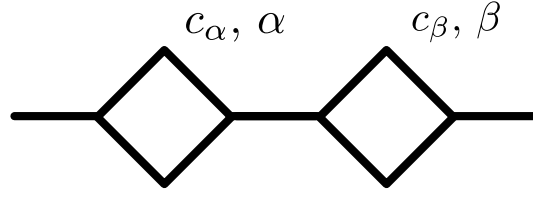

### Constitutive equation

$$\sigma(t) + \frac{c_\alpha}{c_\beta} \frac{d^{\alpha-\beta} \sigma(t)}{dt^{\alpha-\beta}} = c_\alpha \frac{d^\alpha \epsilon(t)}{dt^\alpha}$$

Assuming  $0 \leq \beta \leq \alpha \leq 1$

### Relaxation modulus

$$G(t) = c_\beta t^{-\beta} E_{\alpha-\beta, 1-\beta} \left( -\frac{c_\beta}{c_\alpha} t^{\alpha-\beta} \right)$$

### Creep modulus

$$J(t) = \frac{1}{c_\alpha \Gamma(1+\alpha)} t^\alpha + \frac{1}{c_\beta \Gamma(1+\beta)} t^\beta$$

### Complex modulus

$$G^*(\omega) = \frac{c_\alpha (i\omega)^\alpha \cdot c_\beta (i\omega)^\beta}{c_\alpha (i\omega)^\alpha + c_\beta (i\omega)^\beta}$$

### Storage modulus

$$G'(\omega) = \frac{(c_\beta \omega^\beta)^2 \cdot c_\alpha \omega^\alpha \cos\left(\alpha \frac{\pi}{2}\right) + (c_\alpha \omega^\alpha)^2 \cdot c_\beta \omega^\beta \cos\left(\beta \frac{\pi}{2}\right)}{(c_\alpha \omega^\alpha)^2 + (c_\beta \omega^\beta)^2 + 2c_\alpha \omega^\alpha \cdot c_\beta \omega^\beta \cos\left((\alpha-\beta) \frac{\pi}{2}\right)}$$

### Loss modulus

$$G''(\omega) = \frac{(c_\beta \omega^\beta)^2 \cdot c_\alpha \omega^\alpha \sin\left(\alpha \frac{\pi}{2}\right) + (c_\alpha \omega^\alpha)^2 \cdot c_\beta \omega^\beta \sin\left(\beta \frac{\pi}{2}\right)}{(c_\alpha \omega^\alpha)^2 + (c_\beta \omega^\beta)^2 + 2c_\alpha \omega^\alpha \cdot c_\beta \omega^\beta \cos\left((\alpha-\beta) \frac{\pi}{2}\right)}$$

---

### Special cases

- Maxwell model:  $\beta = 0$  and  $\alpha = 1$

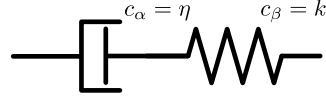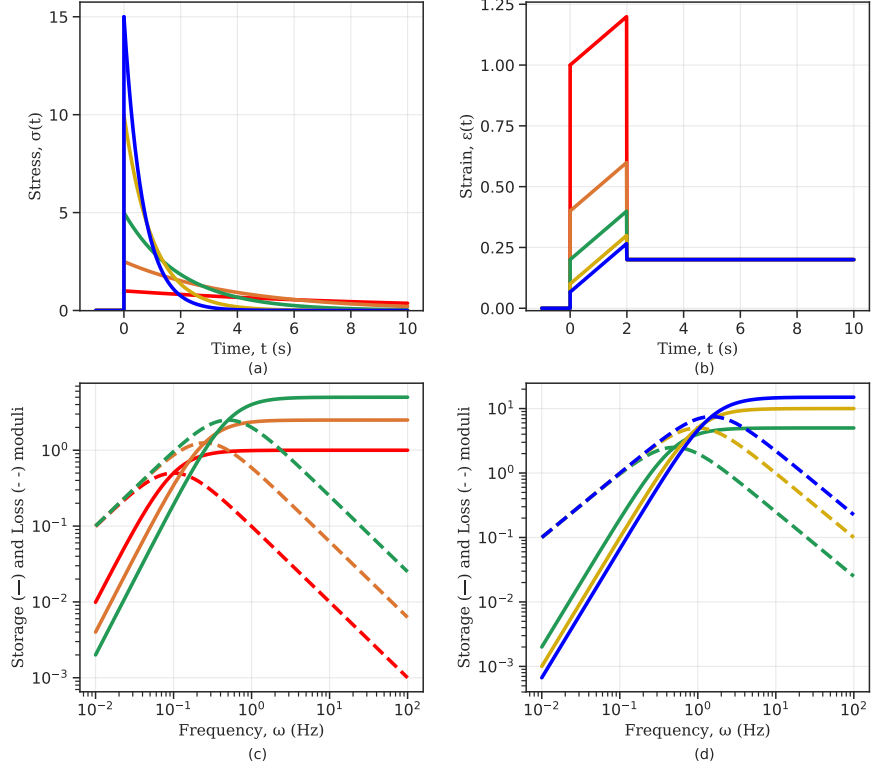

Figure 2: Maxwell model behaviour with  $\eta = 10$  for varying  $k$ . Color reference  $k$  values are red (1.0), orange (2.5), yellow (5.0), green (10.0) and blue (15.0). (a) Relaxation response to step loading. (b) Creep response to step loading and unloading. (c) and (d) Storage (solid line) and loss (dashed line) moduli for the main values of  $\alpha$  with colors ascribed above.

- $\beta = 0$

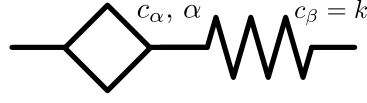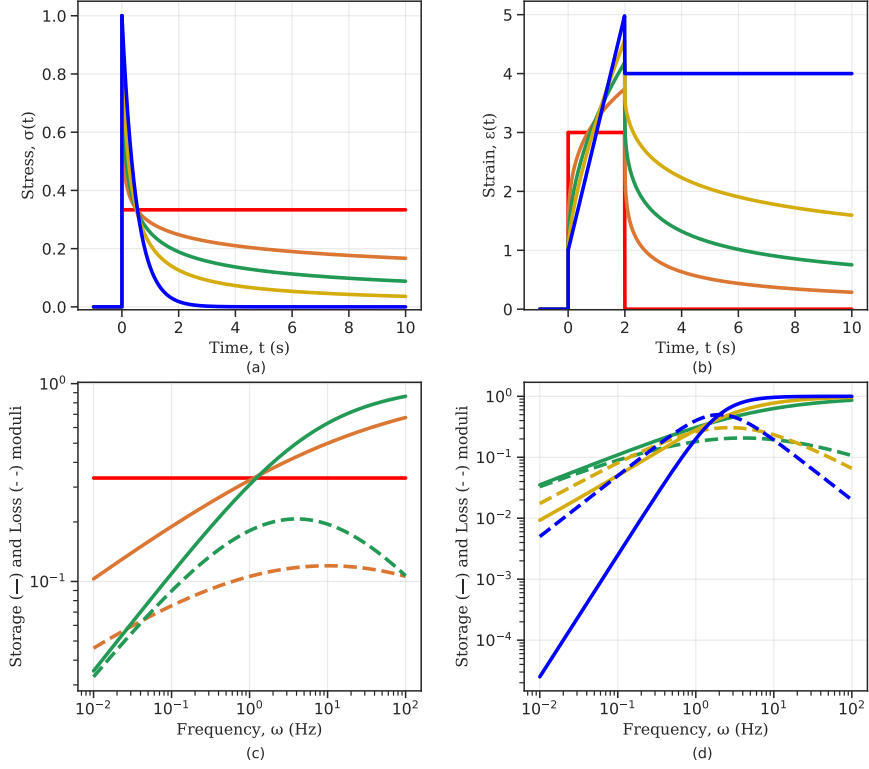

Figure 3: Fractional Maxwell behaviour with  $\beta = 0$  for varying  $\alpha$  ( $c_\alpha = 0.5$  and  $k = 1$ ). Color reference  $\alpha$  values are red (0.1), orange (0.3), yellow (0.5), green (0.7) and blue (0.9). (a) Relaxation response to step loading. (b) Creep response to step loading and unloading. (c) and (d) Storage (solid line) and loss (dashed line) moduli for the main values of  $\alpha$  with colors ascribed above.

- $\alpha = 1$

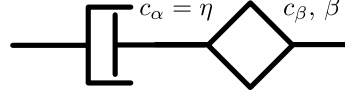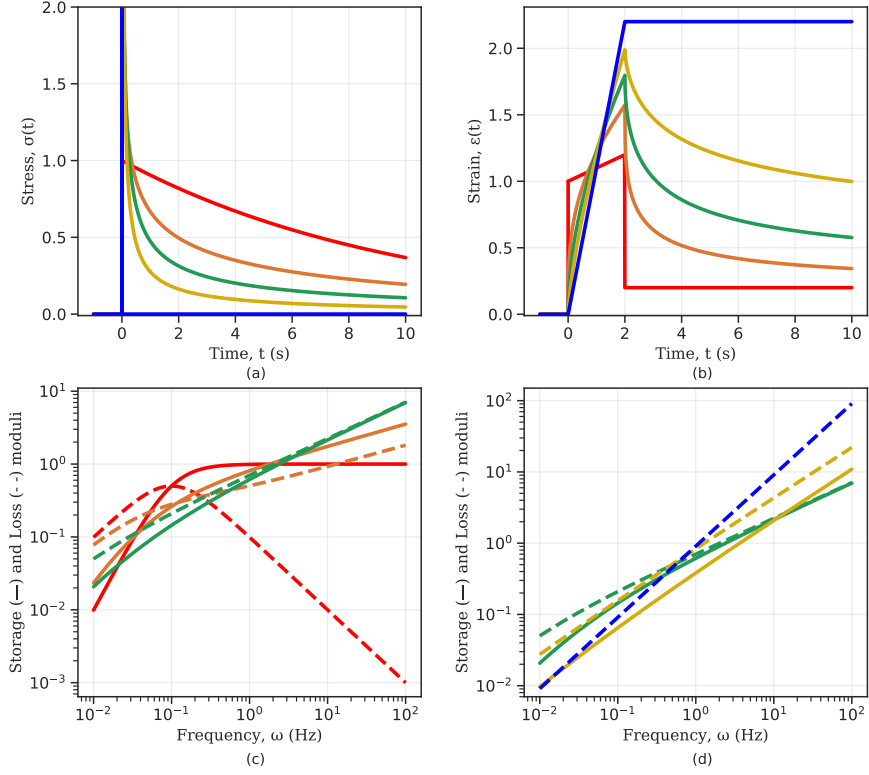

Figure 4: Fractional Maxwell behaviour with  $\alpha = 1$  for varying  $\beta$  ( $\eta = 10$  and  $c_\beta = 1.0$ ). Color reference  $\beta$  values are red (0.1), orange (0.3), yellow (0.5), green (0.7) and blue (0.9). (a) Relaxation response to step loading. (b) Creep response to step loading and unloading. (c) and (d) Storage (solid line) and loss (dashed line) moduli for the main values of  $\beta$  with colors ascribed above.

### 3 Fractional Kelvin-Voigt model

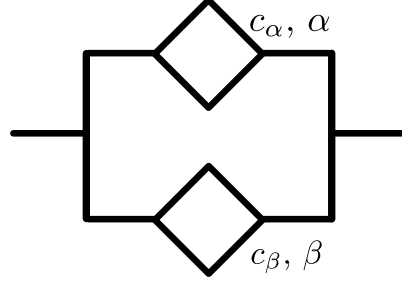

#### Constitutive equation

$$\sigma(t) = c_\alpha \frac{d^\alpha \epsilon(t)}{dt^\alpha} + c_\beta \frac{d^\beta \epsilon(t)}{dt^\beta}$$

Assuming  $0 \leq \beta \leq \alpha \leq 1$

#### Relaxation modulus

$$G(t) = \frac{c_\alpha}{\Gamma(1-\alpha)} t^{-\alpha} + \frac{c_\beta}{\Gamma(1-\beta)} t^{-\beta}$$

#### Creep modulus

$$J(t) = \frac{t^\alpha}{c_\alpha} E_{\alpha-\beta, 1+\alpha} \left( -\frac{c_\beta}{c_\alpha} t^{\alpha-\beta} \right)$$

#### Complex modulus

$$G^*(\omega) = c_\alpha (i\omega)^\alpha + c_\beta (i\omega)^\beta$$

#### Storage modulus

$$G'(\omega) = c_\alpha \omega^\alpha \cos\left(\alpha \frac{\pi}{2}\right) + c_\beta \omega^\beta \cos\left(\beta \frac{\pi}{2}\right)$$

#### Loss modulus

$$G''(\omega) = c_\alpha \omega^\alpha \sin\left(\alpha \frac{\pi}{2}\right) + c_\beta \omega^\beta \sin\left(\beta \frac{\pi}{2}\right)$$



### Special cases

- Kelvin-Voigt model:  $\beta = 0$  and  $\alpha = 1$

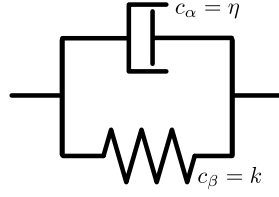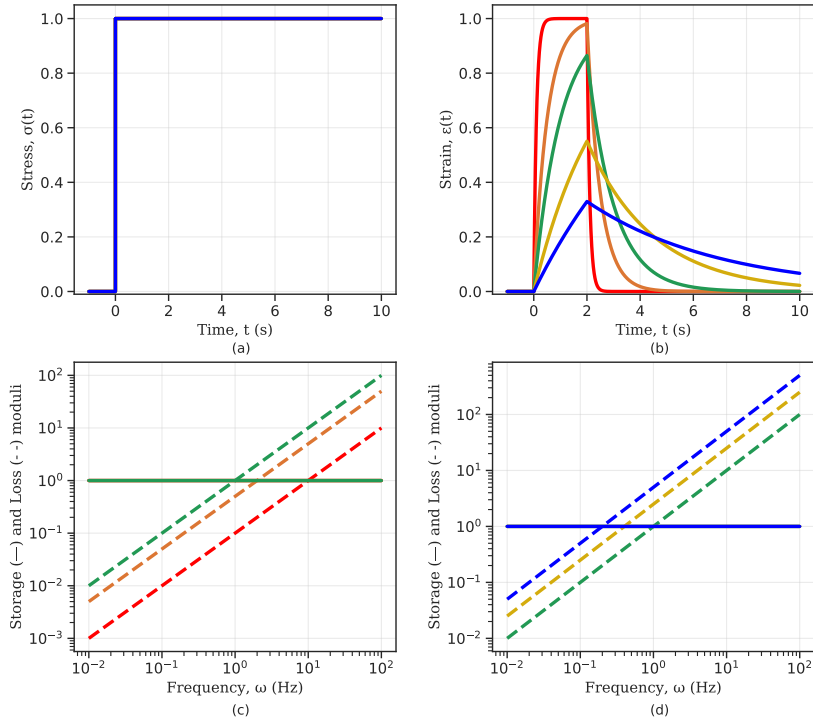

Figure 5: Kelvin-Voigt behaviour with  $k = 1$  for varying  $\eta$ . Color reference  $\eta$  values are red (0.1), orange (0.5), yellow (1.0), green (2.5) and blue (5.0). (a) Relaxation response to step loading. (b) Creep response to step loading and unloading. (c) and (d) Storage (solid line) and loss (dashed line) moduli for the main values of  $\alpha$  with colors ascribed above.

- $\beta = 0$

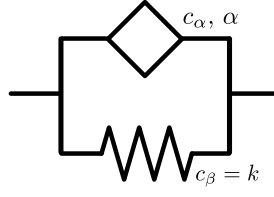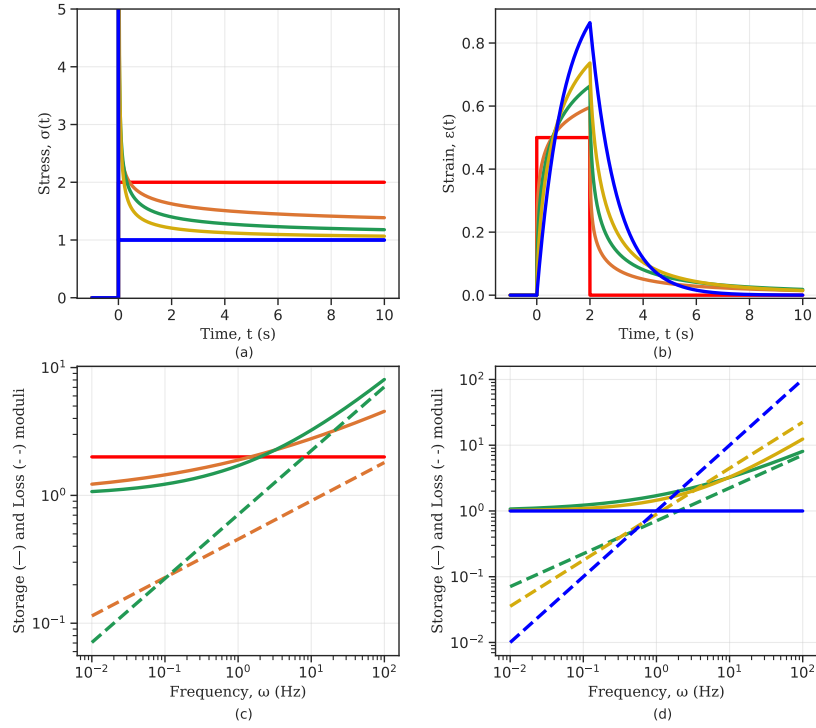

Figure 6: Fractional Kelvin-Voigt behaviour with  $\beta = 0$  for varying  $\alpha$  ( $c_\alpha = 1$  and  $k = 1$ ). Color reference  $\alpha$  values are red (0.0), orange (0.3), yellow (0.5), green (0.7) and blue (1.0). (a) Relaxation response to step loading. (b) Creep response to step loading and unloading. (c) and (d) Storage (solid line) and loss (dashed line) moduli for the main values of  $\alpha$  with colors ascribed above.

- $\alpha = 1$

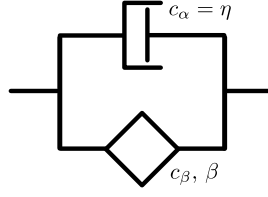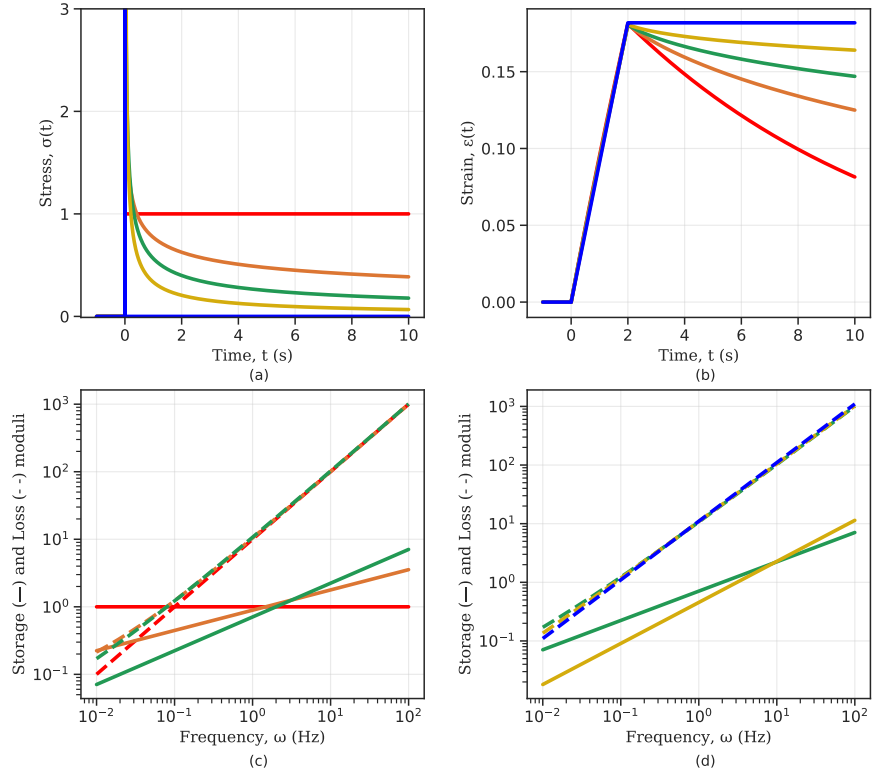

Figure 7: Fractional Kelvin-Voigt behaviour with  $\alpha = 1$  for varying  $\beta$  ( $\eta = 10$  and  $c_\beta = 1$ ). Color reference  $\beta$  values are red (0.0), orange (0.3), yellow (0.5), green (0.7) and blue (1.0). (a) Relaxation response to step loading. (b) Creep response to step loading and unloading. (c) and (d) Storage (—) and loss (---) moduli for the main values of  $\beta$  with colors ascribed above.

## 4 Fractional Zener model

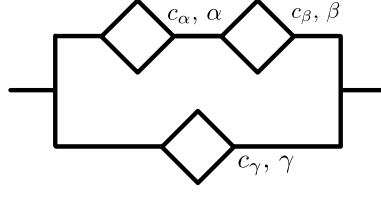

### Constitutive equation

$$\sigma(t) + \frac{c_\alpha}{c_\beta} \frac{d^{\alpha-\beta} \sigma(t)}{dt^{\alpha-\beta}} = c_\alpha \frac{d^\alpha \epsilon(t)}{dt^\alpha} + c_\gamma \frac{d^\gamma \epsilon(t)}{dt^\gamma} + \frac{c_\alpha c_\gamma}{c_\beta} \frac{d^{\alpha+\gamma-\beta} \epsilon(t)}{dt^{\alpha+\gamma-\beta}}$$

Assuming  $0 \leq \beta \leq \alpha \leq 1$

### Relaxation modulus

$$G(t) = c_\beta t^{-\beta} E_{\alpha-\beta, 1-\beta} \left( -\frac{c_\beta}{c_\alpha} t^{\alpha-\beta} \right) + \frac{c_\gamma}{\Gamma(1-\gamma)} t^{-\gamma}$$

### Creep modulus

$$\tilde{J}(s) = \frac{1}{s} \frac{c_\alpha s^\alpha + c_\beta s^\beta}{c_\alpha s^\alpha c_\beta s^\beta + c_\gamma s^\gamma (c_\alpha s^\alpha + c_\beta s^\beta)}$$

### Complex modulus

$$G^*(\omega) = \frac{c_\alpha (i\omega)^\alpha \cdot c_\beta (i\omega)^\beta}{c_\beta (i\omega)^\beta + c_\alpha (i\omega)^\alpha} + c_\gamma (i\omega)^\gamma$$

### Storage modulus

$$G'(\omega) = \frac{(c_\beta \omega^\beta)^2 \cdot c_\alpha \omega^\alpha \cos(\alpha \frac{\pi}{2}) + (c_\alpha \omega^\alpha)^2 \cdot c_\beta \omega^\beta \cos(\beta \frac{\pi}{2})}{(c_\alpha \omega^\alpha)^2 + (c_\beta \omega^\beta)^2 + 2c_\alpha \omega^\alpha \cdot c_\beta \omega^\beta \cos((\alpha-\beta) \frac{\pi}{2})} + c_\gamma \omega^\gamma \cos(\gamma \frac{\pi}{2})$$

### Loss modulus

$$G''(\omega) = \frac{(c_\beta \omega^\beta)^2 \cdot c_\alpha \omega^\alpha \sin(\alpha \frac{\pi}{2}) + (c_\alpha \omega^\alpha)^2 \cdot c_\beta \omega^\beta \sin(\beta \frac{\pi}{2})}{(c_\alpha \omega^\alpha)^2 + (c_\beta \omega^\beta)^2 + 2c_\alpha \omega^\alpha \cdot c_\beta \omega^\beta \cos((\alpha-\beta) \frac{\pi}{2})} + c_\gamma \omega^\gamma \sin(\gamma \frac{\pi}{2})$$

### Special cases

- Standard Linear Solid model:  $\alpha = 1$  and  $\beta = \gamma = 0$

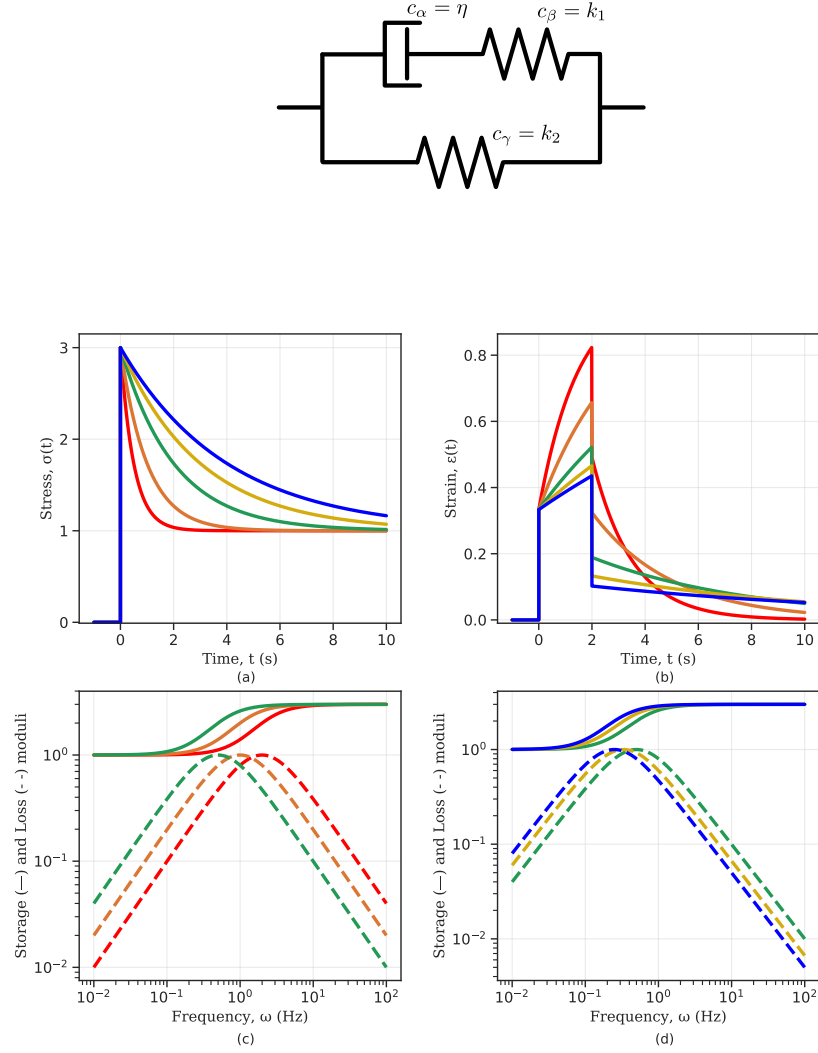

Figure 8: Standard Linear Solid model behaviour with  $\alpha = 1$ ,  $\beta = 0$ ,  $\gamma = 0$  for varying  $\eta$  ( $k_1 = 2$  and  $k_2 = 1$ ). Color reference  $\eta$  values are red (1.0), orange (2.0), yellow (4.0), green (6.0) and blue (8.0). (a) Relaxation response to step loading. (b) Creep response to step loading and unloading. (c) and (d) Storage (solid line) and loss (dashed line) moduli for the main values of  $\alpha$  with colors ascribed above.

- $\beta = \gamma = 0$

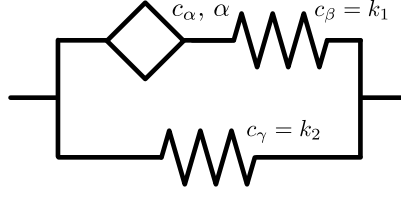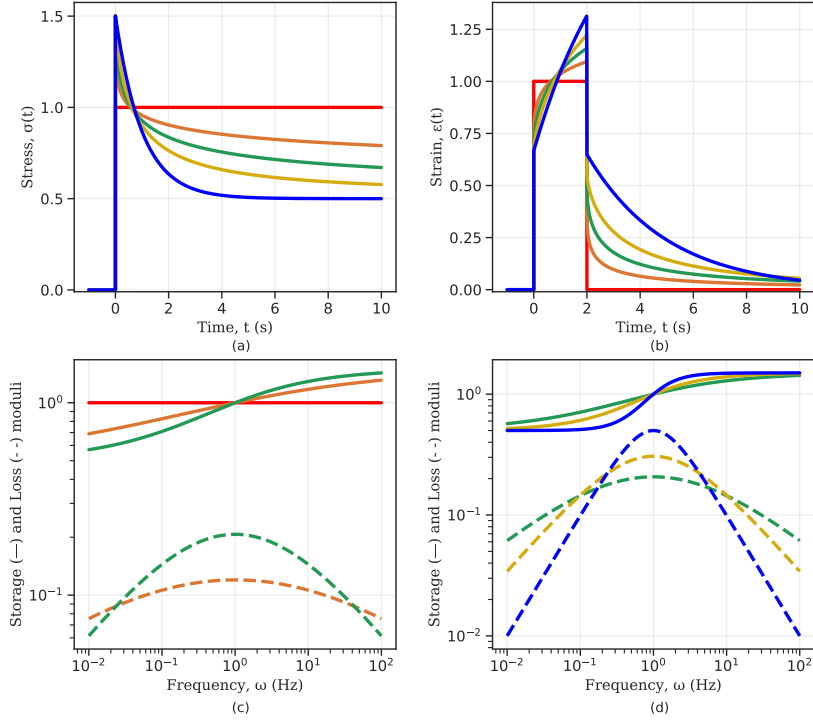

Figure 9: Fractional Zener behaviour with  $\beta = 0$ ,  $\gamma = 0$  for varying  $\alpha$  ( $c_\alpha = 1$ ,  $k_1 = 1$  and  $k_2 = 0.5$ ). Color reference  $\alpha$  values are red (0.0), orange (0.3), yellow (0.5), green (0.7) and blue (1.0). (a) Relaxation response to step loading. (b) Creep response to step loading and unloading. (c) and (d) Storage (solid line) and loss (dashed line) moduli for the main values of  $\alpha$  with colors ascribed above.

- Jeffreys model:  $\alpha = \gamma = 1$  and  $\beta = 0$

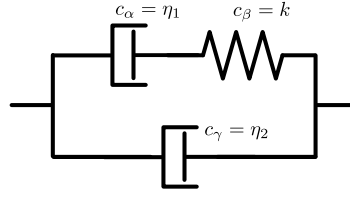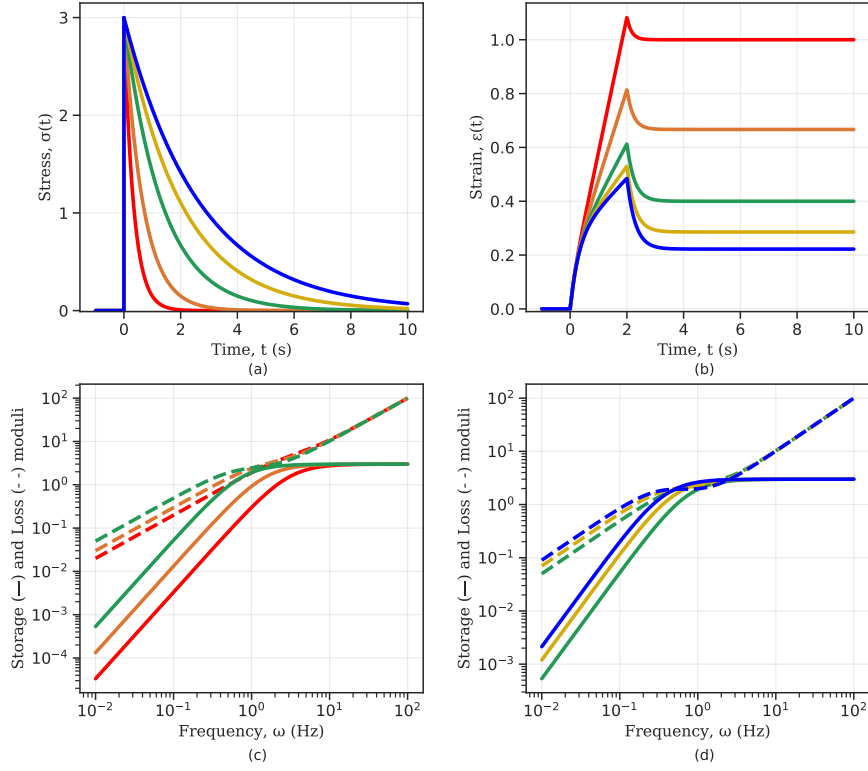

Figure 10: Jeffreys model behaviour for varying  $\eta_1$  ( $k = 3$  and  $\eta_2 = 1$ ). Color reference  $\eta_1$  values are red (1.0), orange (2.0), yellow (4.0), green (6.0) and blue (8.0). (a) Relaxation response to step loading. (b) Creep response to step loading and unloading. (c) and (d) Storage (solid line) and loss (dashed line) moduli for the main values of  $\beta$  with colors ascribed above.

- $\alpha = \gamma = 1$

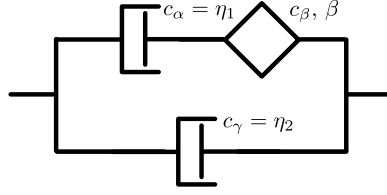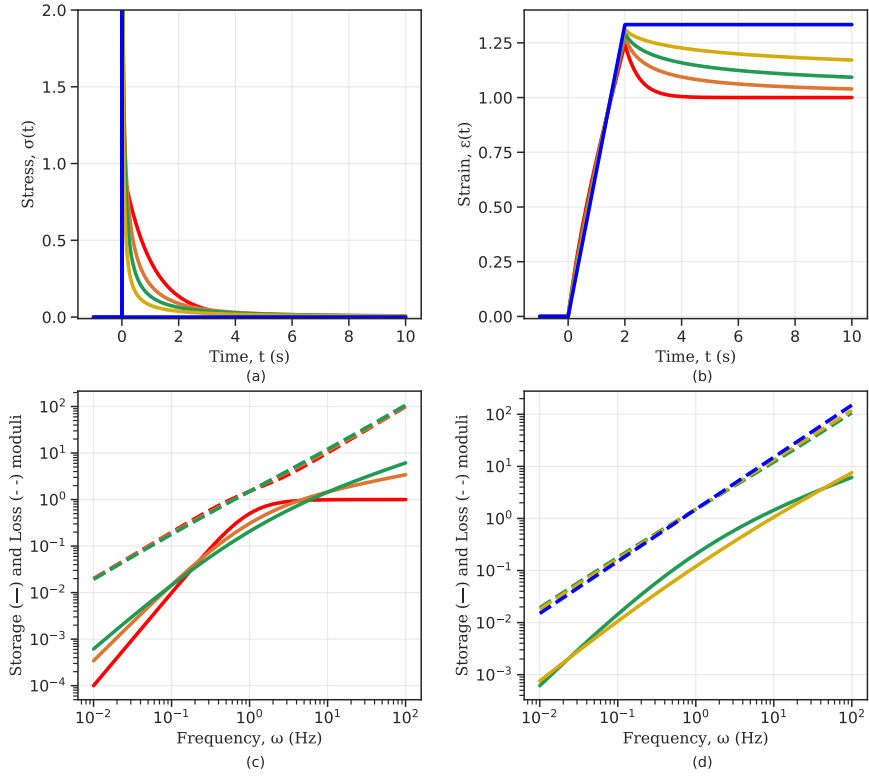

Figure 11: Fractional Zener behaviour with  $\alpha = 1$ ,  $\gamma = 1$  for varying  $\beta$  ( $\eta_1 = 1$ ,  $c_\beta = 1$  and  $\eta_2 = 1$ ). Color reference  $\beta$  values are red (0.0), orange (0.3), yellow (0.5), green (0.7) and blue (1.0). (a) Relaxation response to step loading. (b) Creep response to step loading and unloading. (c) and (d) Storage (—) and loss (---) moduli for the main values of  $\beta$  with colors ascribed above.



- Fractional Zener model:  $\alpha = 1$  and  $\gamma = 0$

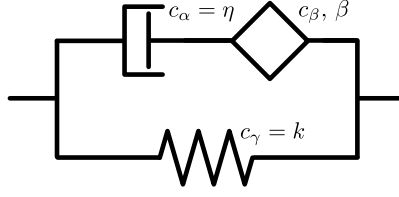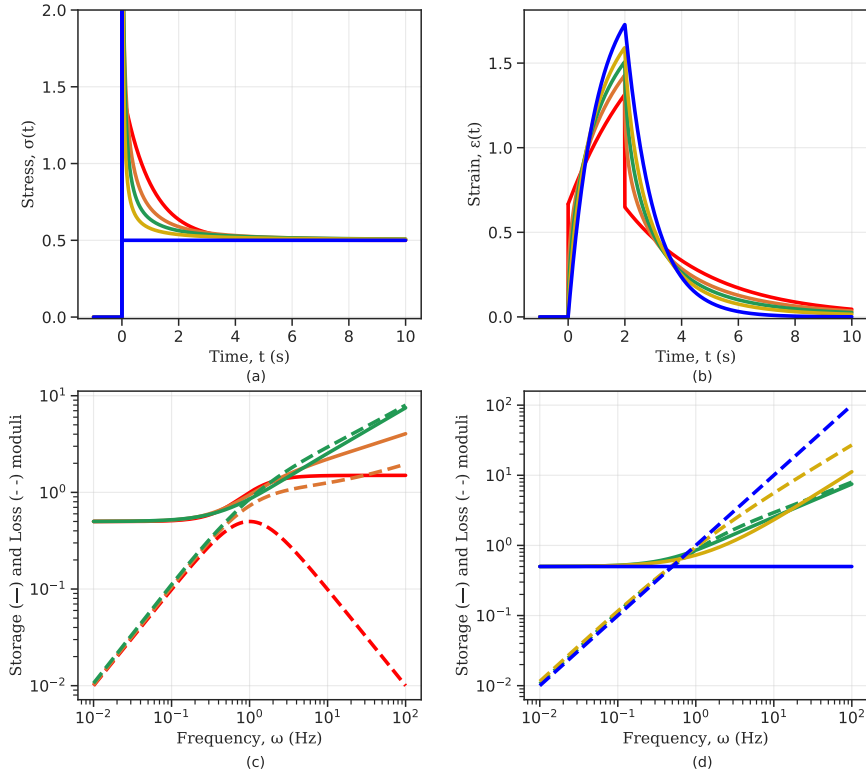

Figure 12: Fractional Solid model behaviour with  $\alpha = 1$ ,  $\gamma = 0$  for varying  $\beta$  ( $\eta = 1$ ,  $c_\beta = 1$ ,  $k = 0.5$ ). Color reference  $\beta$  values are red (0.0), orange (0.3), yellow (0.5), green (0.7) and blue (1.0). (a) Relaxation response to step loading. (b) Creep response to step loading and unloading. (c) and (d) Storage (—) and loss (---) moduli for the main values of  $\beta$  with colors ascribed above.

- $\gamma = \alpha$  or  $\gamma = \beta$

It is then possible to demonstrate that the constitutive equation of the Zener and that of the Poynting-Thomson model presented in the next section are equivalent.

For  $\gamma = \alpha$  the constitutive equation of the Zener model is

$$\sigma(t) + \frac{c_\alpha^Z}{c_\beta^Z} \frac{d^{\alpha-\beta} \sigma(t)}{dt^{\alpha-\beta}} = (c_\alpha^Z + c_\gamma^Z) \frac{d^\alpha \epsilon(t)}{dt^\alpha} + \frac{c_\alpha^Z c_\gamma^Z}{c_\beta^Z} \frac{d^{2\alpha-\beta} \epsilon(t)}{dt^{2\alpha-\beta}}, \quad (1)$$

whereas the constitutive equation of the Poynting-Thomson is

$$\sigma(t) + \frac{c_\alpha^{\text{PT}} + c_\gamma^{\text{PT}}}{c_\beta^{\text{PT}}} \frac{d^{\alpha-\beta} \sigma(t)}{dt^{\alpha-\beta}} = c_\gamma^{\text{PT}} \frac{d^\alpha \epsilon(t)}{dt^\alpha} + \frac{c_\alpha^{\text{PT}} c_\gamma^{\text{PT}}}{c_\beta^{\text{PT}}} \frac{d^{2\alpha-\beta} \epsilon(t)}{dt^{2\alpha-\beta}}. \quad (2)$$

Note that the superscript Z refers to the parameters of the Zener model while PT to those of the Poynting-Thomson model. By equating the coefficients of the terms in equation 1 and 2 we can relate the parameters of the Zener model to those of the Poynting-Thomson model

$$\begin{aligned} c_\alpha^{\text{PT}} &= \frac{c_\gamma^Z (c_\alpha^Z + c_\gamma^Z)}{c_\alpha^Z} \\ c_\beta^{\text{PT}} &= \frac{c_\beta^Z (c_\alpha^Z + c_\gamma^Z)^2}{(c_\alpha^Z)^2} \\ c_\gamma^{\text{PT}} &= c_\alpha^Z + c_\gamma^Z \end{aligned} \quad (3)$$

Therefore, we can calculate the creep modulus from the equivalent Poynting-Thomson model.

For  $\gamma = \beta$  we simply need to exchange  $\alpha$  and  $\beta$  in equation 3 for both PT and Z parameters.

## 5 Fractional Poynting-Thomson model

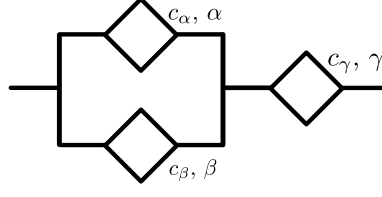

### Constitutive equation

$$\sigma(t) + \frac{c_\alpha}{c_\gamma} \frac{d^{\alpha-\gamma} \sigma(t)}{dt^{\alpha-\gamma}} + \frac{c_\beta}{c_\gamma} \frac{d^{\beta-\gamma} \sigma(t)}{dt^{\beta-\gamma}} = c_\alpha \frac{d^\alpha \epsilon(t)}{dt^\alpha} + c_\beta \frac{d^\beta \epsilon(t)}{dt^\beta}$$

Assuming  $0 \leq \beta \leq \alpha \leq 1$

### Relaxation modulus

$$\tilde{G}(s) = \frac{1}{s} \frac{c_\gamma s^\gamma \cdot [c_\alpha s^\alpha + c_\beta s^\beta]}{c_\gamma s^\gamma + c_\alpha s^\alpha + c_\beta s^\beta}$$

### Creep modulus

$$J(t) = \frac{t^\alpha}{c_\alpha} E_{\alpha-\beta, 1+\alpha} \left( -\frac{c_\beta}{c_\alpha} t^{\alpha-\beta} \right) + \frac{1}{c_\gamma \Gamma(1+\gamma)} t^\gamma$$

### Complex modulus

$$G^*(\omega) = \frac{c_\gamma (i\omega)^\gamma \cdot [c_\alpha (i\omega)^\alpha + c_\beta (i\omega)^\beta]}{c_\gamma (i\omega)^\gamma + c_\alpha (i\omega)^\alpha + c_\beta (i\omega)^\beta}$$

### Storage modulus

$$G'(\omega) = \frac{c_\gamma \omega^\gamma \cos\left(\gamma \frac{\pi}{2}\right) [(c_\alpha \omega^\alpha)^2 + (c_\beta \omega^\beta)^2] + (c_\gamma \omega^\gamma)^2 [c_\alpha \omega^\alpha \cos\left(\alpha \frac{\pi}{2}\right) + c_\beta \omega^\beta \cos\left(\beta \frac{\pi}{2}\right)] + c_\alpha \omega^\alpha \cdot c_\beta \omega^\beta \cdot c_\gamma \omega^\gamma [\cos((\alpha-\beta-\gamma) \frac{\pi}{2}) + \cos((\beta-\alpha-\gamma) \frac{\pi}{2})]}{(c_\alpha \omega^\alpha)^2 + (c_\beta \omega^\beta)^2 + (c_\gamma \omega^\gamma)^2 + 2c_\alpha \omega^\alpha \cdot c_\beta \omega^\beta \cos((\alpha-\beta) \frac{\pi}{2}) + 2c_\alpha \omega^\alpha \cdot c_\gamma \omega^\gamma \cos((\alpha-\gamma) \frac{\pi}{2}) + 2c_\beta \omega^\beta \cdot c_\gamma \omega^\gamma \cos((\beta-\gamma) \frac{\pi}{2})}$$

### Loss modulus

$$G''(\omega) = \frac{c_\gamma \omega^\gamma \sin\left(\gamma \frac{\pi}{2}\right) [(c_\alpha \omega^\alpha)^2 + (c_\beta \omega^\beta)^2] + (c_\gamma \omega^\gamma)^2 [c_\alpha \omega^\alpha \sin\left(\alpha \frac{\pi}{2}\right) + c_\beta \omega^\beta \sin\left(\beta \frac{\pi}{2}\right)] + c_\alpha \omega^\alpha \cdot c_\beta \omega^\beta \cdot c_\gamma \omega^\gamma [\sin((\alpha-\beta-\gamma) \frac{\pi}{2}) + \sin((\beta-\alpha-\gamma) \frac{\pi}{2})]}{(c_\alpha \omega^\alpha)^2 + (c_\beta \omega^\beta)^2 + (c_\gamma \omega^\gamma)^2 + 2c_\alpha \omega^\alpha \cdot c_\beta \omega^\beta \cos((\alpha-\beta) \frac{\pi}{2}) + 2c_\alpha \omega^\alpha \cdot c_\gamma \omega^\gamma \cos((\alpha-\gamma) \frac{\pi}{2}) + 2c_\beta \omega^\beta \cdot c_\gamma \omega^\gamma \cos((\beta-\gamma) \frac{\pi}{2})}$$

### Special cases

- Standard Linear Solid model:  $\alpha = 1$  and  $\beta = \gamma = 0$

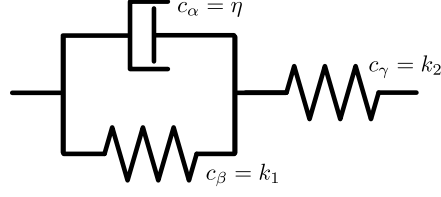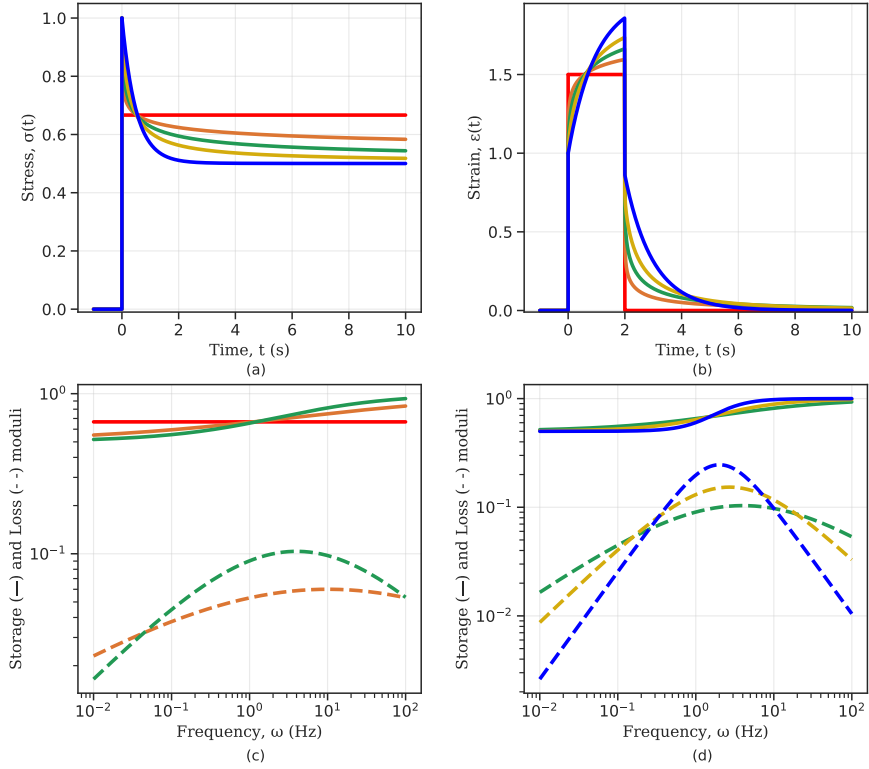

Figure 13: Standard Linear Solid model behaviour for varying  $k_1$  ( $\eta = 1$ ,  $k_2 = 4$ ). Color reference  $k_1$  values are red (1.0), orange (2.0), yellow (3.0), green (4.0) and blue (5.0). (a) Relaxation response to step loading. (b) Creep response to step loading and unloading. (c) and (d) Storage (solid line) and loss (dashed line) moduli for the main values of  $\beta$  with colors ascribed above.

- Jeffreys model:  $\alpha = \gamma = 1$  and  $\beta = 0$

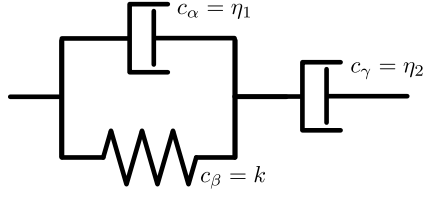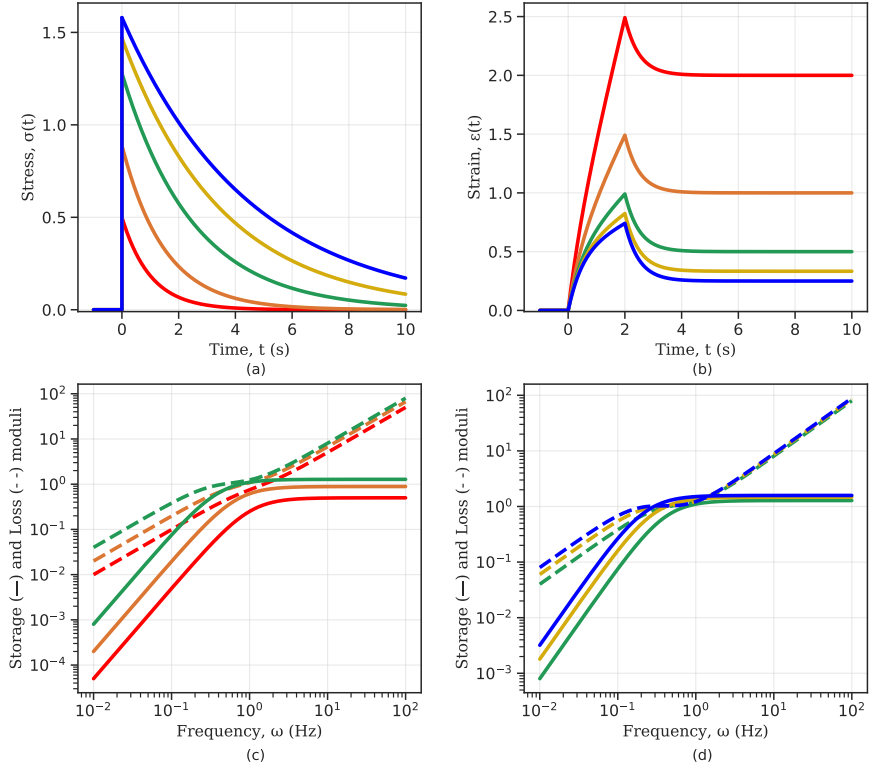

Figure 14: Jeffreys model behaviour for varying  $\eta_2$  ( $\eta_1 = 1$ ,  $k = 2$ ). Color reference  $\eta_2$  values are red (1.0), orange (2.0), yellow (4.0), green (6.0) and blue (8.0). (a) Relaxation response to step loading. (b) Creep response to step loading and unloading. (c) and (d) Storage (solid line) and loss (dashed line) moduli for the main values of  $\beta$  with colors ascribed above.

- $\beta = \gamma = 0$

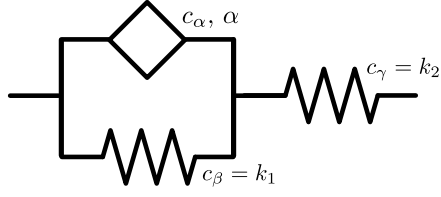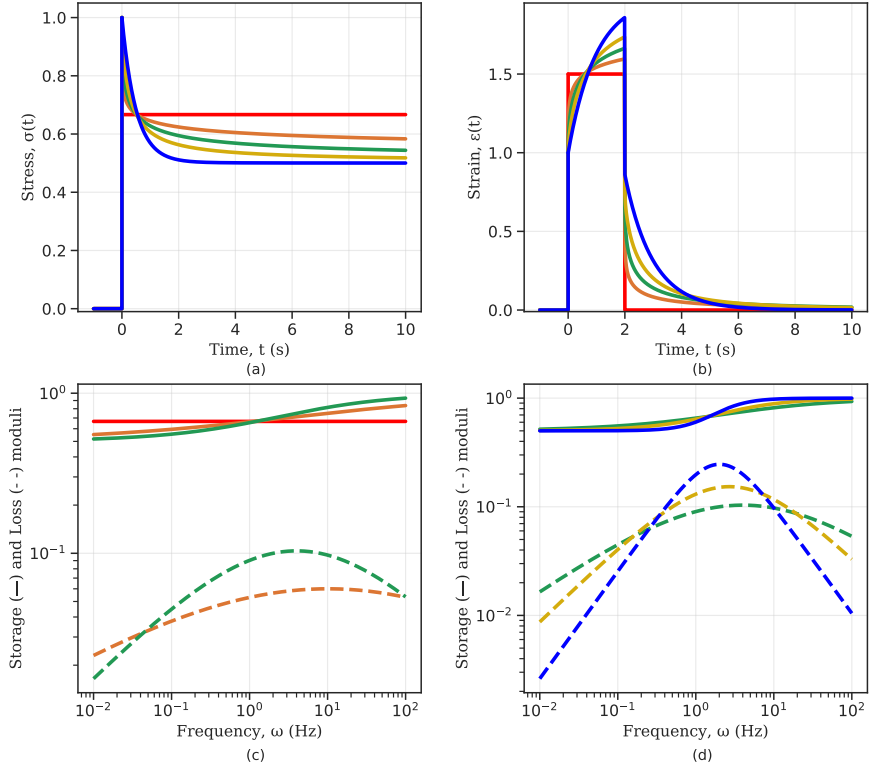

Figure 15: Fractional Poynting-Thomson model behaviour for varying  $\alpha$  ( $c_\alpha = 1$ ,  $k_1 = 1$ ,  $k_2 = 1$ ). Color reference  $\alpha$  values are red (0.0), orange (0.3), yellow (0.5), green (0.7) and blue (1.0). (a) Relaxation response to step loading. (b) Creep response to step loading and unloading. (c) and (d) Storage (solid line) and loss (dashed line) moduli for the main values of  $\beta$  with colors ascribed above.

- $\alpha = \gamma = 1$

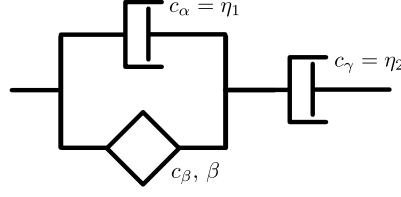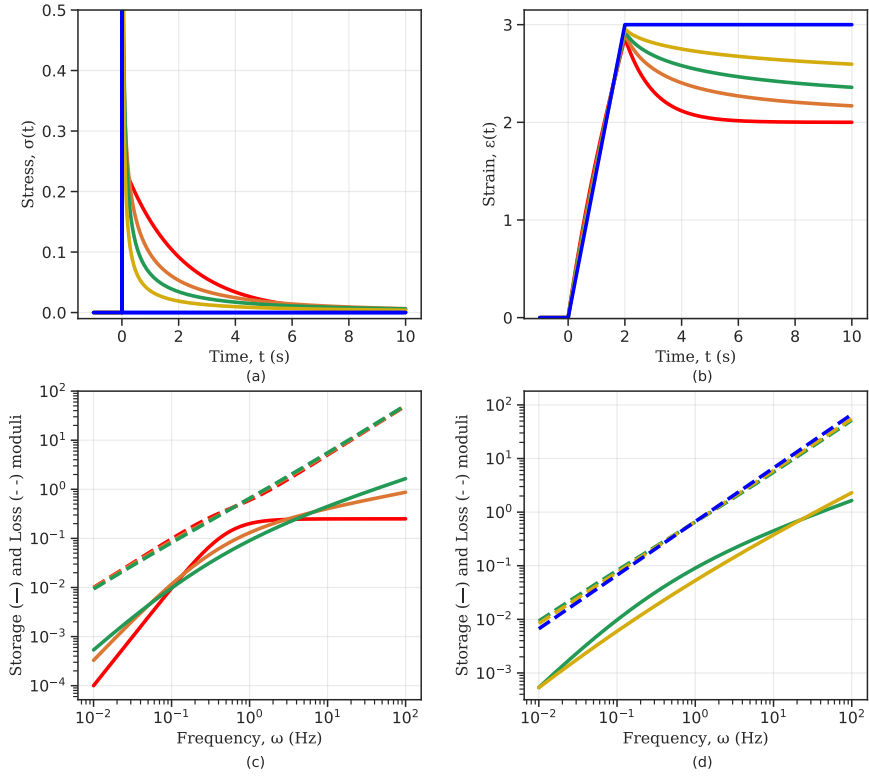

Figure 16: Fractional Poynting-Thomson model behaviour for varying  $\alpha$  ( $\eta_1 = 1$ ,  $c_\beta = 1$ ,  $c_\gamma = 1$ ). Color reference  $\alpha$  values are red (0.0), orange (0.3), yellow (0.5), green (0.7) and blue (1.0). (a) Relaxation response to step loading. (b) Creep response to step loading and unloading. (c) and (d) Storage (solid line) and loss (dashed line) moduli for the main values of  $\beta$  with colors ascribed above.

- $\gamma = \alpha$  or  $\gamma = \beta$

In this case, it is possible to demonstrate that the constitutive equation of the Poynting-Thomson and that of the Zener model are equivalent.

For  $\gamma = \alpha$  the constitutive equation of the Poynting-Thomson model is

$$\sigma(t) + \frac{c_{\alpha}^{\text{PT}}}{c_{\gamma}^{\text{PT}}} \frac{d^{\alpha-\gamma} \sigma(t)}{dt^{\alpha-\gamma}} + \frac{c_{\beta}^{\text{PT}}}{c_{\gamma}^{\text{PT}}} \frac{d^{\beta-\gamma} \sigma(t)}{dt^{\beta-\gamma}} = c_{\alpha}^{\text{PT}} \frac{d^{\alpha} \epsilon(t)}{dt^{\alpha}} + c_{\beta}^{\text{PT}} \frac{d^{\beta} \epsilon(t)}{dt^{\beta}}. \quad (4)$$

By taking the  $\alpha - \beta$ -th derivative of the equation and multiplying both sides by  $c_{\gamma}^{\text{PT}}/c_{\beta}^{\text{PT}}$  we obtain

$$\sigma(t) + \frac{c_{\alpha}^{\text{PT}} + c_{\gamma}^{\text{PT}}}{c_{\beta}^{\text{PT}}} \frac{d^{\alpha-\beta} \sigma(t)}{dt^{\alpha-\beta}} = c_{\gamma}^{\text{PT}} \frac{d^{\alpha} \epsilon(t)}{dt^{\alpha}} + \frac{c_{\alpha}^{\text{PT}} c_{\gamma}^{\text{PT}}}{c_{\beta}^{\text{PT}}} \frac{d^{2\alpha-\beta} \epsilon(t)}{dt^{2\alpha-\beta}}; \quad (5)$$

whereas the constitutive equation of the Zener model becomes

$$\sigma(t) + \frac{c_{\alpha}^{\text{Z}}}{c_{\beta}^{\text{Z}}} \frac{d^{\alpha-\beta} \sigma(t)}{dt^{\alpha-\beta}} = (c_{\alpha}^{\text{Z}} + c_{\gamma}^{\text{Z}}) \frac{d^{\alpha} \epsilon(t)}{dt^{\alpha}} + \frac{c_{\alpha}^{\text{Z}} c_{\gamma}^{\text{Z}}}{c_{\beta}^{\text{Z}}} \frac{d^{2\alpha-\beta} \epsilon(t)}{dt^{2\alpha-\beta}}. \quad (6)$$

Note that the superscript PT refers to the parameters of the Poynting-Thomson model while Z to those of the Zener model. By equating the coefficients of the terms in equation 5 and 6 we can relate the parameters of the Poynting-Thomson model to those of the Zener

$$\begin{aligned} c_{\alpha}^{\text{Z}} &= \frac{(c_{\gamma}^{\text{PT}})^2}{c_{\alpha}^{\text{PT}} + c_{\gamma}^{\text{PT}}} \\ c_{\beta}^{\text{Z}} &= \frac{c_{\beta}^{\text{PT}} (c_{\gamma}^{\text{PT}})^2}{(c_{\alpha}^{\text{PT}} + c_{\gamma}^{\text{PT}})^2} \\ c_{\gamma}^{\text{Z}} &= \frac{c_{\alpha}^{\text{PT}} c_{\gamma}^{\text{PT}}}{c_{\alpha}^{\text{PT}} + c_{\gamma}^{\text{PT}}} \end{aligned} \quad (7)$$

Therefore, we can calculate the relaxation modulus from the equivalent Zener model.

For  $\gamma = \beta$  we simply need to exchange  $\alpha$  and  $\beta$  in equation 7 for both PT and Z parameters.
